# Supplementary material for: Role of surface termination in the metal-insulator transition of V$_2$O$_3$(0001) ultrathin films
Source: arXiv:2106.08555 source file (2021-06-16)
Supplement: Supplementary file 1 [file Supporting_Information.pdf]

Supporting Information

# Role of surface termination in the metal-insulator transition of $V_2O_3$(0001) ultrathin films

Asish K. Kundu[1, 2, *], Sukanta Barman[1, 3], and Krishnakumar S. R. Menon[1, ‡]

[1]Surface Physics and Material Science Division, Saha Institute of Nuclear Physics, HBNI, 1/AF Bidhannagar, Kolkata 700064, India
[2] Condensed Matter Physics and Materials Science Department, Brookhaven National Laboratory, Upton, New York 11973, USA
[3] Department of Physics, Raja Peary Mohan College, Uttarpara, Hooghly 712258, India

*asishkumar2008@gmail.com
‡ krishna.menon@saha.ac.in

## EDCs: above and below MIT for V=O terminated surface:

In figure S1, we have fitted EDCs to understand how the individual components (QP and LHB) of V 3*d* bands change across MIT. In figure S1 (a), peak 'a' represents the LHB and peak 'b' represents the QP peak. For the simplicity of fitting, we do not account the Fermi function convolution, instead, we have used another inverted peak 'c' to account for the peak shape near the Fermi level. Fitting results are summarized in table S1. The QP peak in the PM phase shifts its spectral weight towards the higher binding energy during transition to the AFI phase, accompanied by strong spectral weight redistribution. It can be seen that the width (FWHM) of the LHB peak changes from 1.4 eV to 1.24 eV by going from PM and AFI phase and shifted towards the higher binding energy by 80 meV. Peak shift is also clearly visible in the raw data itself (main text figure 4(a) and (b)). These energy shifts and FWHM change of LHB across MIT strongly suggest that the correlation (*U/W*) strength gets enhanced in the AFI phase than the PM phase.

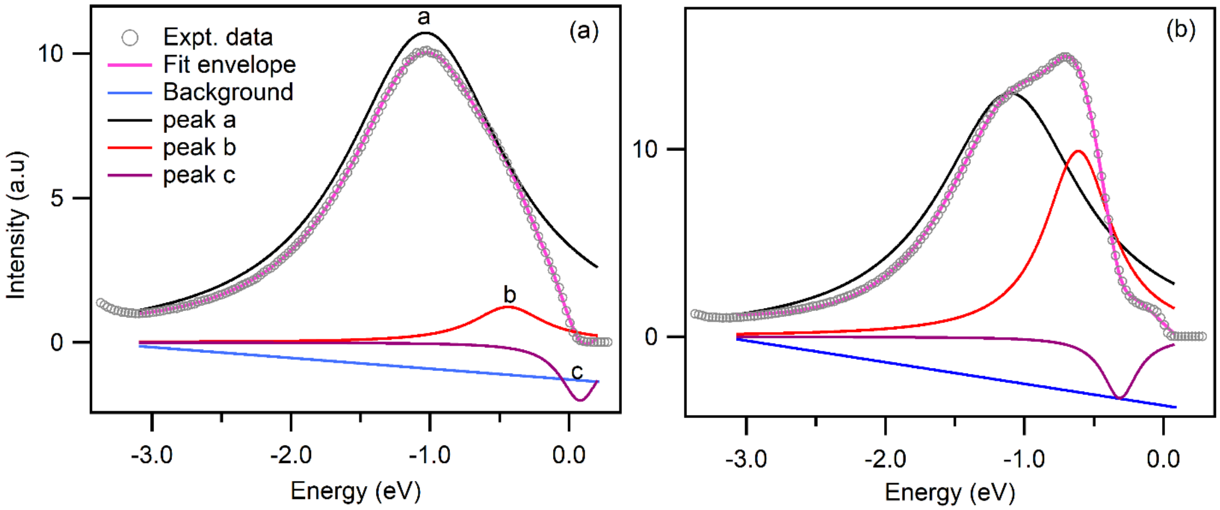


Figure S1. EDCs (a) above (300 K) and (b) below (108 K) MIT temperature for V=O terminated surface. Both the spectra were normalized at background (-3.0 eV). EDCs were fitting using a linear background and three Lorentzian peaks. The 'a' and 'b' peaks were used to capture the QP and LHB peak and 'c' (inverted Lorentzian peak) is used to better account the spectral shape near the Fermi level.

| Temperature | LHB | | | | QP | | | |
|---|---|---|---|---|---|---|---|---|
| | Position (eV) | FWHM (eV) | Area (a.u) | Amplitude (a.u) | Position (eV) | FWHM (eV) | Area (a.u) | Amplitude (a.u) |
| 300 K | -1.03 | 1.4 | 0.93 | 0.82 | -0.42 | 0.62 | 0.05 | 0.1 |
| 108 K | -1.11 | 1.24 | 1.0 | 1.0 | -0.62 | 0.58 | 0.36 | 0.76 |

Table S1. Summarizing the fitting results of Fig. S1. Area and amplitude values of peaks are normalized *w.r.t* the LHB values of 108 K spectra.

## Comparison of He-I and He-II EDCs for V=O terminated surface:

Figure S2 shows the comparison of EDCs between He-I and He-II for the V=O terminated surface. It can be seen that the relative intensity of the Fermi edge-like feature at the Fermi level (0 eV) increases in He-II spectra compared to He-I. This clearly suggest that the edge-like features have surface related origin as He-II is more surface sensitive than He-I.

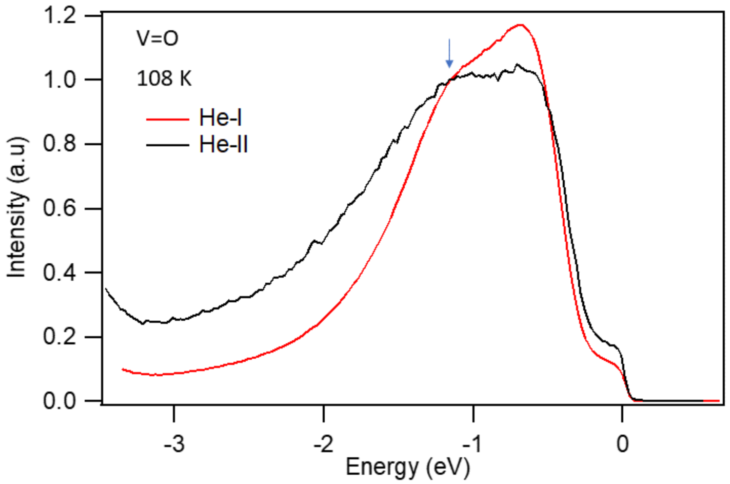


Figure S2. Comparison of EDCs between He-I (21.2 eV) and He-II (40.8 eV) using photons at 108 K for the V=O terminated surface (grown at P($O_2$ )= $2\times10^{-7}$ mbar, 600 K and followed by UHV annealed at 773 K). Both the spectra are normalized at the peak position of lower Hubbard band (indicated by arrow).

## EDCs of as-grown and UHV annealed $V_2O_3$ films along with Ag(111) for comparison:

In figure S3, change in spectral features between as-grown and UHV annealed films are clearly visible, both in the V 3*d* and O 2*p* region. Upon UHV annealing, a similar enhancement of spectral features was reported by Schoiswohl *et al.* [24]. According to them, these changes suggest the formation of large-area V2O3 (0001) islands with the surface terminated by well-ordered V=O groups. In agreement, we also observe the Fermi-edge-like feature (inset of figure S3) which we speculate (see main text) originating from V=O surface layers, are also increases. By comparing with the Ag(111)spectra, possibilities of Ag segregation from substrate or formation of micro-cracks in the film can be ruled out, as no intensity enhancement of Ag related peaks are observed in figure S3.

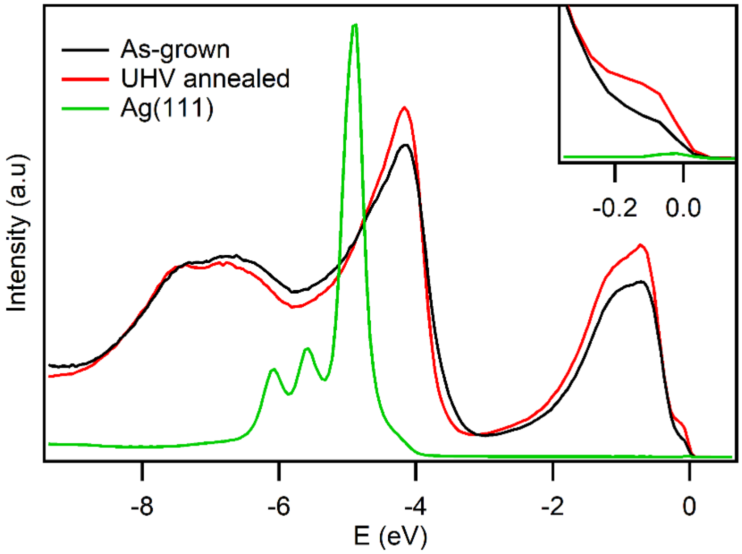


Figure S3. EDCs of as-grown ($P(O_2) = 2\times10^{-7}$ mbar and substrate temperature of 600 K) and UHV annealed (773 K) $V_2O_3$(0001) films along with Ag(111) for comparison. Inset shows zoomed-in view near the Fermi energy. All the data were collected at 108 K.
